# Supplementary material for: Vcc: Scaling Transformers to 128K Tokens or More by Prioritizing Important Tokens
Source: arXiv:2305.04241 source file (2023-05-27)
Supplement: Supplementary file 1 [file appendix.tex]

% \documentclass{article}


% % if you need to pass options to natbib, use, e.g.:
% %     \PassOptionsToPackage{numbers, compress}{natbib}
% % before loading neurips_2023

% \PassOptionsToPackage{numbers, compress}{natbib}

% % ready for submission
% \usepackage{neurips_2023}


% % to compile a preprint version, e.g., for submission to arXiv, add add the
% % [preprint] option:
% %     \usepackage[preprint]{neurips_2023}


% % to compile a camera-ready version, add the [final] option, e.g.:
% %     \usepackage[final]{neurips_2023}


% % to avoid loading the natbib package, add option nonatbib:
% %    \usepackage[nonatbib]{neurips_2023}


% \usepackage[utf8]{inputenc} % allow utf-8 input
% \usepackage[T1]{fontenc}    % use 8-bit T1 fonts
% \usepackage{hyperref}       % hyperlinks
% \usepackage{url}            % simple URL typesetting
% \usepackage{booktabs}       % professional-quality tables
% \usepackage{amsfonts}       % blackboard math symbols
% \usepackage{nicefrac}       % compact symbols for 1/2, etc.
% \usepackage{microtype}      % microtypography
% \usepackage{xcolor}         % colors
% \usepackage{graphicx}
% \usepackage{amsmath}
% \usepackage{amssymb}
% \usepackage{mathtools}
% \usepackage{amsthm}
% \usepackage{wrapfig}
% \usepackage{float}

% \usepackage{algorithm}
% \usepackage{algorithmic}
% \usepackage{color, colortbl}
% \definecolor{LightCyan}{rgb}{0.88,1,1}
% \definecolor{Gray}{gray}{0.9}
% \definecolor{twitterblue}{rgb}{0.113,0.631,0.949}
% \definecolor{arrowcolor1}{rgb}{0.11, 0.69, 0}
% \definecolor{arrowcolor2}{rgb}{1, 0.26, 0.63}
% \definecolor{arrowcolor3}{rgb}{0.57, 0.57, 0.57}
% \definecolor{cgreen}{rgb}{0.38, 0.85, 0.21}

% \theoremstyle{plain}
% \newtheorem{theorem}{Theorem}[section]
% \newtheorem{proposition}[theorem]{Proposition}
% \newtheorem{lemma}[theorem]{Lemma}
% \newtheorem{corollary}[theorem]{Corollary}
% \newtheorem{claim}[theorem]{Claim}
% \theoremstyle{definition}
% \newtheorem{definition}[theorem]{Definition}
% \newtheorem{assumption}[theorem]{Assumption}
% \theoremstyle{remark}
% \newtheorem{remark}[theorem]{Remark}


% \input{symbols}
% \input{enable_comments}

% \title{Appendix: VCC: Scaling Transformers to 128K Tokens or More by Prioritizing Important Tokens}


% % The \author macro works with any number of authors. There are two commands
% % used to separate the names and addresses of multiple authors: \And and \AND.
% %
% % Using \And between authors leaves it to LaTeX to determine where to break the
% % lines. Using \AND forces a line break at that point. So, if LaTeX puts 3 of 4
% % authors names on the first line, and the last on the second line, try using
% % \AND instead of \And before the third author name.


% \author{%
%   Zhanpeng Zeng \\
%   % Department of Computer Sciences \\
%   University of Wisconsin, Madison \\
%   % Madison, WI 53706 \\
%   \texttt{zzeng38@wisc.edu} \\
% \And
%   Cole Hawkins \\
%   AWS AI \\
%   % New York, NY 10001 \\
%   \texttt{colehawk@amazon.com} \\
% \And
%   Mingyi Hong \\
%   % Department of Electrical and Computer Engineering \\
%   University of Minnesota, Minneapolis \\
%   % Minneapolis, MN 55455 \\
%   \texttt{mhong@umn.edu} \\
% \And
%   Aston Zhang \\
%   AWS AI \\
%   % Palo Alto, CA 94303 \\
%   \texttt{astonz@amazon.com} \\
% \And
%   Nikolaos Pappas \\
%   AWS AI \\
%   % Palo Alto, CA 94303 \\
%   \texttt{nppappa@amazon.com} \\
% \And
%   Vikas Singh \\
%   % Department of Computer Sciences \\
%   University of Wisconsin, Madison \\
%   % Madison, WI 53706 \\
%   \texttt{vsingh@biostat.wisc.edu} \\
% \And
%   Shuai Zheng \\
%   AWS AI \\
%   % Palo Alto, CA 94303 \\
%   \texttt{shzheng@amazon.com} \\
% }


% \begin{document}


% \maketitle


% \section{Definition of Notations}
% \label{ap:notations}
% \input{tables/notation_table}

% We provide a table \ref{tab:notation_table} of notations that are used for more than once so that the readers can refer to their definition easily. 

% \section{Details of Multi-Resolution Compression}
% \label{ap:mrc_details}
% \input{appendix/mrc_details}

% \section{Details of Proposed Data Structure}
% \label{ap:cache_details}
% \input{appendix/cache_details}

% \section{Complexity Analysis}
% \label{ap:complexity}
% \input{appendix/complexity}

% \section{Potential Application to Decoders}
% \label{ap:apply_decoder}
% \input{appendix/apply_decoder}

% \section{Experiments}
% \label{ap:experiment}
% \input{appendix/experiment_details}

% \section{Practical Questions}
% \label{ap:questions}
% \input{appendix/misc}

% \bibliography{main}
% \bibliographystyle{plain}

% \end{document}
